# Supplementary material for: First-principles multiscale modelling of charged adsorbates on doped graphene
Source: arXiv:1609.04328 source file (2017-03-27)
Supplement: Supplementary file 1 [file supplementary_material.pdf]

arXiv [cond-mat.mes-hall]

Supplementary Material for:  
 First-principles multiscale modelling of charged adsorbates on doped graphene  
 Fabiano Corsetti, Arash A. Mostofi, Johannes Lischner

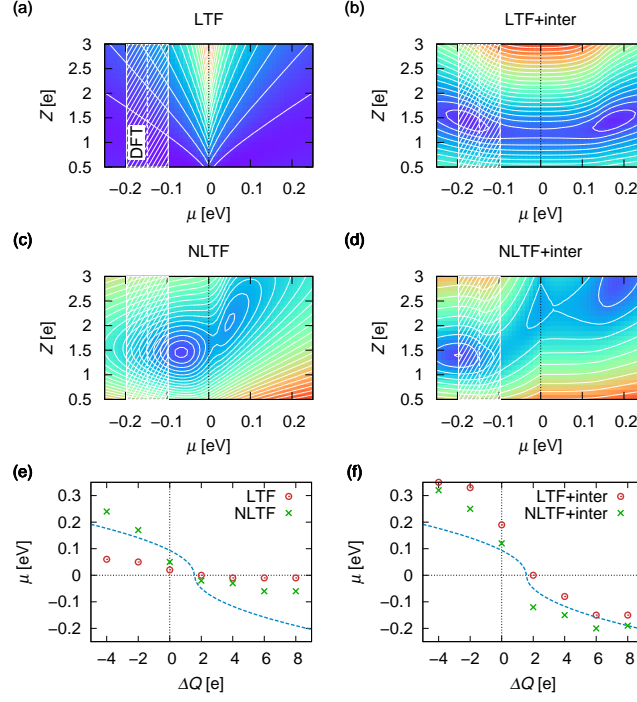

FIG. S1. Fitting of the four screening models to the DFT self-consistent potential. The models are explained in the main text. (a-d) Fitness metric  $\mathcal{F}$  contour plot for each model for the case of  $\Delta Q = 6$  e, as a function of the adatom charge  $Z$  and the graphene chemical potential  $\mu$ . The dashed vertical line shows the value of the chemical potential estimated from the DFT DOS (Fig. 2 in the main text), and the hatched region shows the range of uncertainty. (e-f) The chemical potential  $\mu$  obtained from the minimum of  $\mathcal{F}$  as a function of supercell charge  $\Delta Q$  for all four models. The linear-bands fit to DFT from Fig. 2 in the main text is also included for comparison.

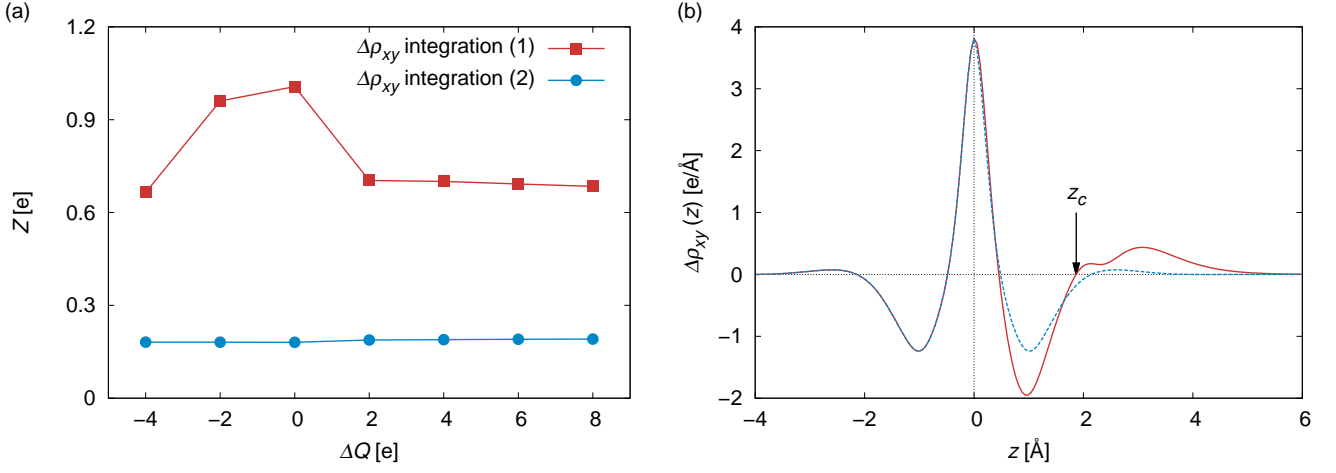

FIG. S2. Charge transfer between a Ca adatom and the graphene substrate from DFT simulations employing the  $xy$  planar-averaged electronic charge-density ( $z$  is perpendicular to the graphene plane). We use the charge-density difference  $\Delta\rho_{xy}$  between the combined adatom+substrate simulation and the separate adatom-only and substrate-only simulations. (a) The charge of the Ca adatom  $Z$  as a function of supercell charge  $\Delta Q$  for two integration schemes. Scheme (1) uses an adatom-substrate cutoff position  $z_c$ , defined to be the root of  $\Delta\rho_{xy}$  in between the graphene plane ( $z = 0$ ) and the Ca position ( $z = 2 \text{ \AA}$ ) closest to the Ca ion; the charge of the ion is then defined as  $Z = \int_{z_c}^{\infty} \Delta\rho_{xy}(z) dz$ . This is the scheme proposed by Chan *et al.* [Phys. Rev. B **77**, 235430 (2008)]. Scheme (2) makes the assumption that the charge-density difference due to free carriers in the system will be symmetric in  $z$  around the graphene plane, and approximates this as  $\Delta\rho_{xy}(-|z|)$ ; the remaining charge is considered to be bound to the Ca ion, and so  $Z = \int_0^{\infty} \Delta\rho_{xy}(z) - \Delta\rho_{xy}(-z) dz$ . (b) The total charge-density difference (solid line) and symmetrized free carrier charge-density (dashed line).

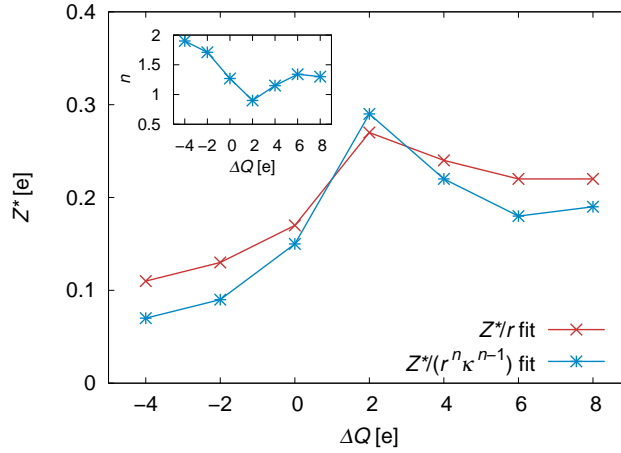

FIG. S3. Fitting of two simple empirical forms to the DFT self-consistent potential as a function of the supercell charge  $\Delta Q$ . The first is  $Z^*/r$ , where  $r$  is the distance from the Ca adatom and  $Z^*$  is the effective screened charge of the ion; the second is  $Z^*/(r^n \kappa^{n-1})$ , where  $n$  is the exponent of the power-law decay and  $\kappa$  is an arbitrary length-scale (set here to  $0.1 a_0$ ). The fitted  $Z^*$  exhibits a sharp maximum at  $\Delta Q = 2$  e, supporting the idea that this is the closest simulation to the undoped case (i.e., the bare impurity charge  $Z \approx 2$  e, making the total free carrier charge  $\Delta Q - Z \approx 0$ ), as both n-/p-doping can be expected to increase the screening and so decrease the effective charge. This is further reinforced by the fitted values of  $n$ , which give a decay of the form  $1/r$  close to  $\Delta Q = 2$  e, and a faster decay on either side of this value. This agrees with the analysis of Katsnelson [Phys. Rev. B **74**, 201401 (2006)] from Thomas-Fermi theory, which predicts a transition from a  $1/r$  decay at small  $r$  to a  $1/r^3$  decay at large  $r$ , with the transition length decreasing with increased doping and tending to infinity for the undoped case.

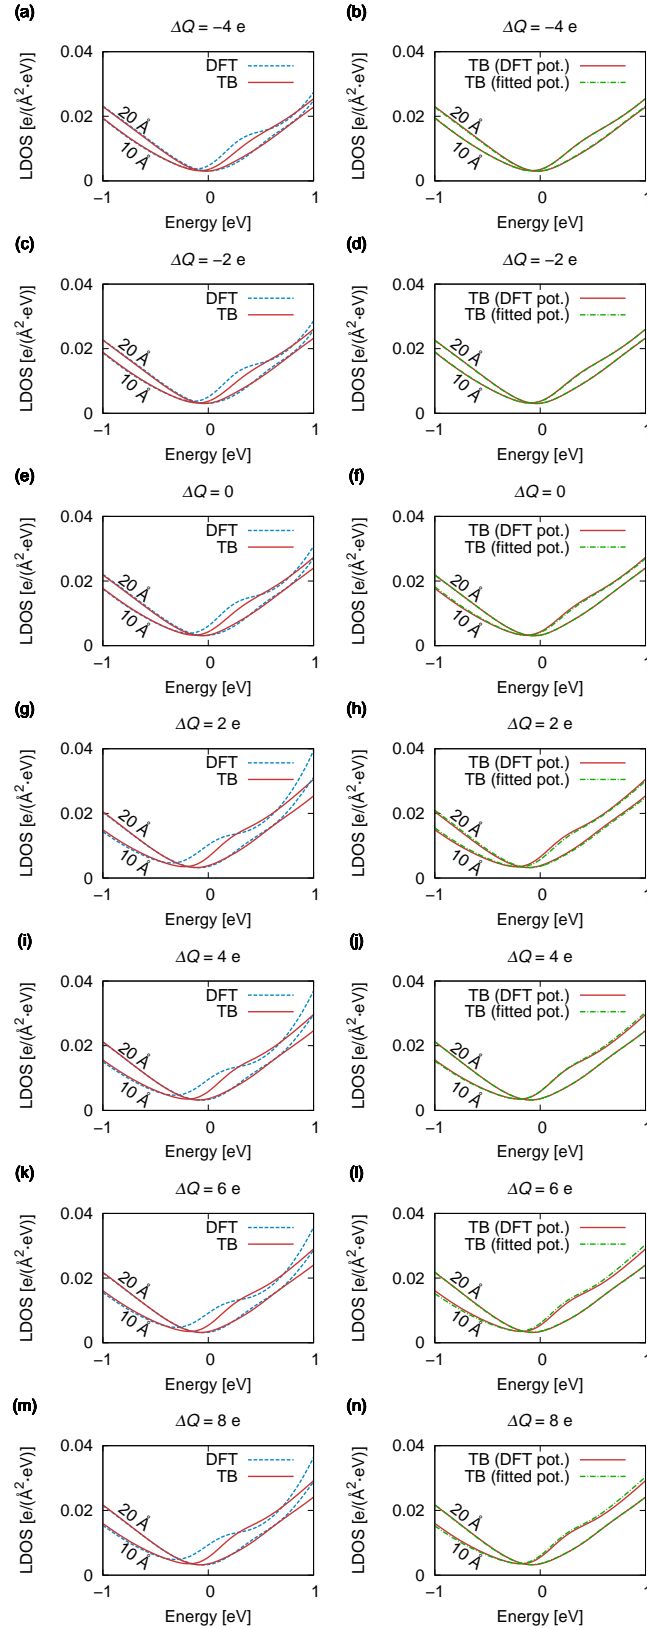

FIG. S4. Comparison of the LDOS at two different distances from the Ca impurity obtained in the same  $56 \times 56$  supercell with three different methods: full DFT, TB with the local on-site potential extracted from DFT, and TB with a screened potential fitted to the DFT one using the NLTF+inter model. The comparison is made for each of the charge states  $\Delta Q$  calculated with DFT (one per row). The left column shows the comparison between the full DFT and the TB with the DFT potential, while the right column shows the comparison between the two TB methods. As can be seen, the difference for the latter is almost not visible on this scale. The discrepancy between DFT and TB is expected to be due mainly to the off-diagonal terms for the screened potential, neglected in our TB model.
